# Supplementary material for: Fast event-driven simulations for soft spheres: from dynamics to Laves phase nucleation
Source: arXiv:2403.12755 ancillary file (2025-10-08)
Supplement: Supplementary file 1 [file SI.pdf]

# Fast event-driven simulations for soft spheres: from dynamics to Laves phase nucleation – Supplemental Information

Antoine Castagnède[1], Laura Filion[2] and Frank Smallenburg[1]
[1] *Université Paris-Saclay, CNRS, Laboratoire de Physique des Solides, 91405 Orsay, France*
[2] *Soft Condensed Matter and Biophysics, Debye Institute of Nanomaterials Science, Utrecht University, Utrecht, Netherlands*

## RANDOM NUMBER GENERATION

A key part of the event-driven Monte Carlo (EDMC) approach is the stochastic determination of collision distances between particles. This requires the generation of a random energy $\Delta U$, drawn from the Boltzmann distribution at the chosen temperature $T$. In other words, we want to generate a random number $x = \beta \Delta U$, with $\beta = 1/k_B T$ the inverse thermal energy, such that its probability distribution is given by

$$P(x) = \exp(-x). \quad (1)$$

There are several algorithms available to do this. Perhaps the most straightforward method is to generate a uniform random number $y$ in the interval $(0, 1]$ and calculate $x = -\log(y)$. However, this approach is relatively slow due to the computational complexity of the logarithm. As a result, using this method we found that random number generation was a significant part of the total computation time of our simulation code.

To improve on this, we instead use an implementation of an algorithm introduced by Ahrens and Dieter [1], which uses on average $1 + \log(2) \simeq 1.693$ uniform random numbers per generated exponential random number [2]. In order to efficiently generate uniform random numbers, we use the Xoshiro256+ algorithm [3].

## VERY LOW TEMPERATURE NUCLEATION TRAJECTORIES

We display in Figure 1 a set of nucleation trajectories for our binary WCA mixture of interest (composition $x_L = 1/3$, size ratio $\gamma = 0.78$) at very low temperature $k_B T/\epsilon = 10^{-4}$ and a range of different densities. Simulations were run independently for at least $6 \times 10^6 \tau_{kT}$ with prior system equilibration of $10^4$ and $10^6 \tau_{kT}$ respectively. This density scan displays four distinct regimes. First, at low density ($\rho\sigma_L^3 = 1.175$), we do not record nucleation events within a reasonable simulation time. Second, for intermediate densities ($1.180 \leq \rho\sigma_L^3 \lesssim 1.188$), we report clear nucleation events to which we can associate induction times. For higher densities ($1.188 \lesssim \rho\sigma_L^3 \leq 1.22$), we observe an immediate onset of crystallization, rather than discrete nucleation events. Finally, for the highest density systems ($1.22 \lesssim \rho$), slow system dynamics prevent crystallization on the time scale of our simulations.

## REFERENCES

[1] J. H. Ahrens and U. Dieter, Communications of the ACM **15**, 873 (1972).
[2] L. Devroye and L. Devroye, Non-Uniform Random Variate Generation pp. 379–484 (1986).
[3] D. Blackman and S. Vigna, ACM Transactions on Mathematical Software (TOMS) **47**, 1 (2021).

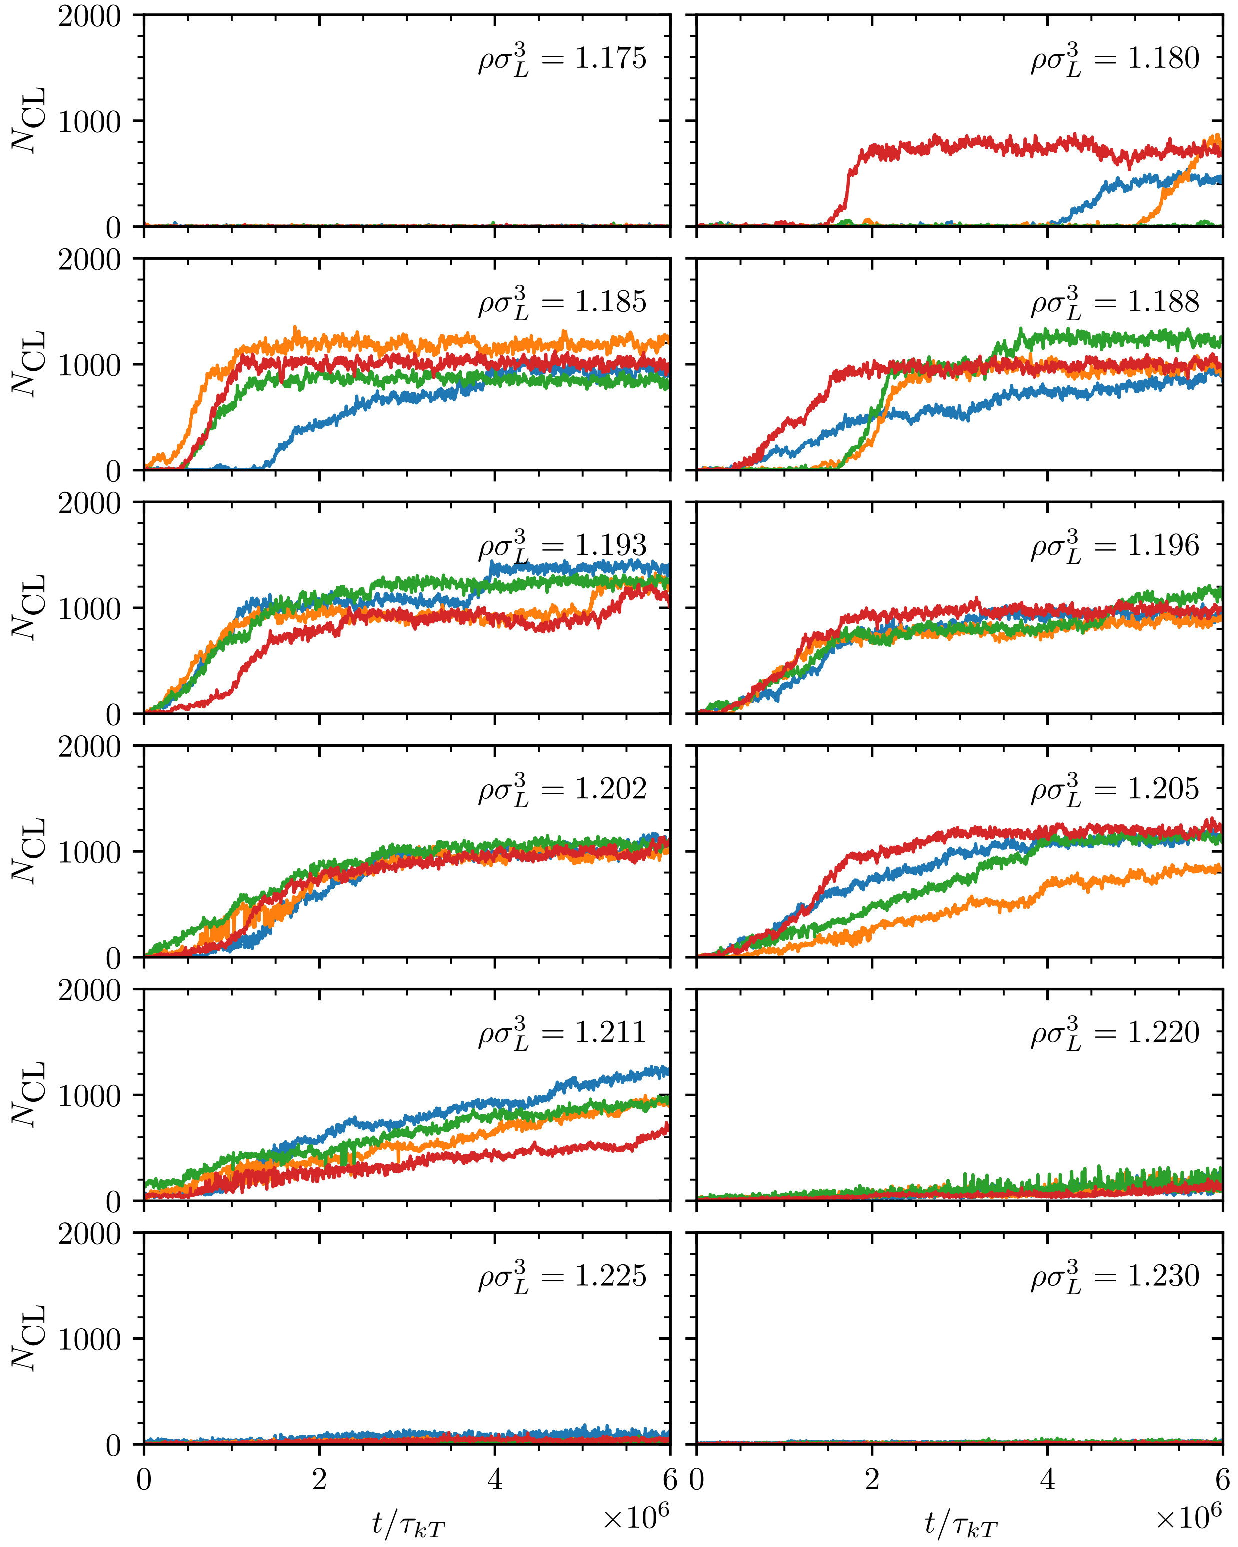


FIG. 1: Nucleation attempts at very low temperature ($k_BT/\epsilon = 10^{-4}$) for the binary WCA system ($x_{\rm L} = 1/3$, $q = 0.78$), showing multiple nucleation events with and without waiting time at state points $\rho\sigma_L^3 = 1.175$ through $\rho\sigma_L^3 = 1.230$. Each system consisted of $N = 2000$ particles.
